# Supplementary material for: DAST: Difficulty-Aware Self-Training on Large Language Models
Source: arXiv:2503.09029 source file (2025-03-12)
Supplement: Supplementary file 1 [file prompt_example.tex]

10 different few-shot prompts for sampling on TriviaQA are demonstrated in Table \ref{table:example}.

\begin{table*}[!ht]
  \centering
  % \resizebox{0.9\linewidth}{!}
  {\begin{tabular}{cp{13cm}}
    \hline
    \textbf{Examplar ID} & \textbf{Examples} \\
    % \hline
    % \rowcolor{platinum}
    % \multicolumn{2}{c}{\textbf{TriviaQA} \\
    \hline
    1 & Q: Which William wrote the novel Lord Of The Flies? A: Golding. \\
    2 & Q: Where in England was Dame Judi Dench born? A: York, UK. \\
    3 & Q: Neil Armstrong was a pilot in which war? A: Korean. \\
    4 & Q: How many home runs did baseball great Ty Cobb hit in the three world series in which he played? A: None. \\
    5 & Q: Who had a big 60s No 1 with Tossin' and Turnin'? A: Bobby Lewis. \\
    6 & Q: Which Disney film had the theme tune A Whole New World? A: 'Ala' ad Din. \\
    7 & Q: In basketball where do the Celtics come from? A: City of Boston. \\
    8 & Q: Which element along with polonium did the Curies discover? A: Radium. \\
    9 & Q: Who was the Egyptian king whose tomb an treasures were discovered in the Valley of the Kings in 1922? A: Tutanhamon. \\
    10 & Q: Where were the 2004 Summer Olympic Games held? A: Atina, Greece. \\
    \hline
  \end{tabular}}
  \caption{Demonstrations of 1-shot examples for TriviaQA sampling to construct \textsc{UAlign} dataset.}
\label{table:example}
\end{table*}

\begin{table*}[!ht]
  \centering
  % \resizebox{0.9\linewidth}{!}
  {\begin{tabular}{cp{13cm}}
    \hline
    \textbf{Examplar ID} & \textbf{Examples} \\
    % \hline
    % \rowcolor{platinum}
    % \multicolumn{2}{c}{\textbf{TriviaQA} \\
    \hline
    1 & Q: What type of organism is commonly used in preparation of foods such as cheese and yogurt? A: mesophilic organisms. \\
    2 & Q: What phenomenon makes global winds blow northeast to southwest or the reverse in the northern hemisphere and northwest to southeast or the reverse in the southern hemisphere? A: coriolis effect. \\
    3 & Q: Changes from a less-ordered state to a more-ordered state (such as a liquid to a solid) are always what? A: exothermic. \\
    4 & Q: What is the least dangerous radioactive decay? A: alpha decay. \\
    5 & Q: Kilauea in hawaii is the world’s most continuously active volcano. very active volcanoes characteristically eject red-hot rocks and lava rather than this? A: smoke and ash. \\
    6 & Q: When a meteoroid reaches earth, what is the remaining object called? A: meteorite. \\
    7 & Q: What kind of a reaction occurs when a substance reacts quickly with oxygen? A: combustion reaction. \\
    8 & Q: Organisms categorized by what species descriptor demonstrate a version of allopatric speciation and have limited regions of overlap with one another, but where they overlap they interbreed successfully? A: ring species. \\
    9 & Q: Alpha emission is a type of what? A: radioactivity. \\
    10 & Q: What is the stored food in a seed called? A: endosperm. \\
    \hline
  \end{tabular}}
  \caption{Demonstrations of 1-shot examples for SciQ sampling to construct \textsc{UAlign} dataset.}
\label{table:example2}
\end{table*}
